# Supplementary material for: No-pumping theorem for many particle stochastic pumps
Source: arXiv:1312.6852 source file (2013-12-24)
Supplement: Supplementary file 1 [file Sup_Mat_1.pdf]

# Supplementary material for No-pumping theorem for many particle stochastic pumps

Shahaf Asban[1] and Saar Rahav[2]

[1]Faculty of Physics ,Technion - Israel Institute of Technology, Haifa 32000, Israel
[2]Schulich Faculty of Chemistry ,Technion - Israel Institute of Technology, Haifa 32000, Israel
(Dated: October 31, 2013)

## I. MORE ON THE STRUCTURE OF NON-INTERACTING STOCHASTIC PUMPS

When a single particle with $k$ sites has the transition rate matrix $\mathcal{R}^{(1)}$, the corresponding non interacting $N$ particle stochastic pump has a transition rate matrix given by the outer product

$$\mathcal{R}^{(N)} = \bigoplus_{i=1}^{N} \mathcal{R}^{(1)}. \tag{1}$$

Here $\bigoplus$ denotes the Kronecker sum. For square matrices of the same dimension this sum is defined by $\mathcal{A} \oplus \mathcal{B} \equiv \mathcal{A} \otimes I + I \otimes \mathcal{B}$, where $\otimes$ is the Kronecker/tensor product. If the graph $\mathcal{G}^{(1)}(v, E)$ is the graph representation the single particle system with $\mathcal{R}^{(1)}$, then graph representing a many particle system (with $\mathcal{R}^{(N)}$) is given by a Cartesian product of the single particle graphs

$$\mathcal{G}^{(N)} = \mathop{\square}_{i=1}^{N} \mathcal{G}^{(1)}, \tag{2}$$

as discussed in the text and depicted in Fig.1 there. $v$ and $E$ denote the vertices and edges of the graph, respectively. Assuming that the long time asymptotic state of the single particle pump is $|p^{(1)}(t)\rangle$, then the corresponding state of the $N$ (non interacting) particle pump is

$$|p^{(N)}(t)\rangle = \bigotimes_{i=1}^{N} |p^{(1)}(t)\rangle. \tag{3}$$

Using this structure, it is easy to verify that the net particle currents for non interacting particles are simply a sum of uncorrelated contributions from the different particles. The single particle instantaneous currents are $J^{(1)}_{\alpha\beta}(t) = R_{\alpha\beta}(t) p_\beta(t) - R_{\beta\alpha}(t) p_\alpha(t)$. A straight forward calculation of the many particle fluxes, using Eqs. (1) and (3) and then summation over the location of spectators (see main text) leads to $J^{(N)}_{\alpha\beta}(t) = N J^{(1)}_{\alpha\beta}(t)$.

## II. DERIVATION OF CONSERVATION LAWS

Let the particle density at site $\sigma$ be

$$\rho_\sigma \equiv \sum_{k=1}^{N} \sum_{\boldsymbol{X}_{|k}} P(x_1, x_2, \cdots, x_{k-1}, \sigma, x_{k+1} \cdots x_N). \tag{4}$$

The summation on the right hand side is over all configurations in which the $k^{th}$ particle location is set to site $\sigma$, as well as over $k$. The total current flowing between sites $\sigma \to \sigma'$ is

$$\Phi_{\sigma \to \sigma'} = \sum_{k=1}^{N} \sum_{\boldsymbol{X}_{|k}} \phi_{\boldsymbol{X}_{|k};\sigma \to \sigma'}. \tag{5}$$

Since the after a long time probability distribution is periodic in time, so is the density, and

$$\oint_T \dot{\rho}_\sigma dt = 0. \tag{6}$$

The conservation laws for the many particle system originate from a similar equation which holds for the probability distribution $P(\mathbf{X})$,

$$0 = \oint_T dt \dot{P}(\mathbf{X}) = -\sum_{k=1}^{N} \sum_{\sigma' \neq x_k} \phi_{\boldsymbol{X}_{|k};x_k \to \sigma'}, \tag{7}$$

or equivalently,

$$0 = \oint_T dt \dot{P}(\mathbf{X}) = \sum_{k=1}^{N} \sum_{\sigma' \neq x_k} \phi_{\boldsymbol{X}_{|k};\sigma' \to x_k}. \tag{8}$$

Substitution of Eq. (4) in Eq. (6) gives

$$0 = \oint_T dt \sum_{k=1}^{N} \sum_{\boldsymbol{X}_{|k}} \dot{P}(x_1, .., x_{k-1}, \sigma, x_{k+1}, .., x_N). \tag{9}$$

With the help of Eq. (8) we get

$$\sum_{k=1}^{N} \sum_{l=1}^{N} \sum_{\boldsymbol{X}_{|kl}} \sum_{\sigma' \neq x_l} \phi_{\boldsymbol{X}_{|kl};x_k=\sigma;\sigma' \to x_l} = 0, \tag{10}$$

where $\boldsymbol{X}_{|kl}$ denote the location of all particles except the $k$'th and $l$'th ones. For $k = l$ $\boldsymbol{X}_{|kl}$ is simply an awkward way to write $\boldsymbol{X}_{|k}$.

We consider the contributions with $k = l$ and $k \neq l$ separately. For $k \neq l$ we note that there is a summation over both $x_l, \sigma$ so these terms appear in pairs of the form $\phi_{\boldsymbol{X}_{|kl};x_k=\sigma;\alpha \to \beta} + \phi_{\boldsymbol{X}_{|kl};x_k=\sigma;\beta \to \alpha}$ which clearly vanish, since they sum the same flux in opposite directions.

The remaining contributions to the density conservation law come from the $k = l$ terms in the sum. This gives

$$\sum_{\sigma' \neq \sigma} \left[ \sum_{k=1}^{N} \sum_{\boldsymbol{X}_{|k}} \phi_{\boldsymbol{X}_{|k};\sigma \to \sigma'} \right] = 0. \tag{11}$$

The summation over $k$ and $\boldsymbol{X}_{|k}$ maps the fluxes into particle currents. We therefore arrive at the conservation laws

$$\oint_T dt \dot{\rho}_\sigma = 0 = \sum_{\sigma' \neq \sigma} \Phi_{\sigma \to \sigma'}. \tag{12}$$

Eq. (12) is what one would have naively have guessed as the conservation law for the density of particles, but it is helpful to verify that it does emerge out of the conservation of probability in the many particle master equation.
